# Supplementary material for: UniIR: Training and Benchmarking Universal Multimodal Information Retrievers
Source: arXiv:2311.17136 source file (2023-11-28)
Supplement: Supplementary file 2 [file appendix.tex]

\section{Appendix}

\subsection{Hyperparameters}
We use the BLIP (\texttt{BLIP/models/model\_large.pth}) and BLIP2 (\texttt{BLIP2/blip2\_pretrained.pt}) models from the LAVIS~\cite{li-etal-2023-lavis} 
library with the supported \texttt{feature\_extractor} function. For SigLIP
(\texttt{timm/ViT-L-16-SigLIP-256}) model we use the Open-CLIP~\cite{ilharco_gabriel_2021_5143773} library.

\input{tables_and_figures/figure_dataset}
\input{tables_and_figures/table_instructions}
\input{tables_and_figures/table_union}
